# Supplementary material for: Linear Precoding Based on Polynomial Expansion: Reducing Complexity in Massive MIMO
Source: arXiv:1310.1806 source file (2014-07-24)
Supplement: Supplementary file 1 [file SecAppendixunified.tex]

\input{SecAppendixresubmitext.tex}
